# Supplementary material for: UMI on Legs: Making Manipulation Policies Mobile with Manipulation-Centric Whole-body Controllers
Source: arXiv:2407.10353 source file (2024-07-14)
Supplement: Supplementary file 1 [file supp.tex]

\documentclass{article}

\usepackage[preprint]{corl_2024} %
\input{packages}

\title{UMI-on-Legs: Making Manipulation Policies Mobile with a Manipulation-Centric Whole-body Controller}

\begin{document}
\maketitle

\tableofcontents
\input{text/supp_text}

\bibliography{main}  %

\end{document}
